# Supplementary material for: Mode transition ($\alpha-\gamma$) and hysteresis in microwave-driven low-temperature plasmas
Source: arXiv:2203.00420 source file (2022-03-01)
Supplement: Supplementary file 1 [file supplementary.tex]

We measured the rotational temperature using a monochromator (DM700 “DongWoo Optron”) and ICCD camera (Pi-MAX 1024i “Princeton Instruments”) to verify the results obtained with the previous OES at a higher precision.

\begin{figure}[h!]
    \centering
    \includegraphics[width = 130 mm]{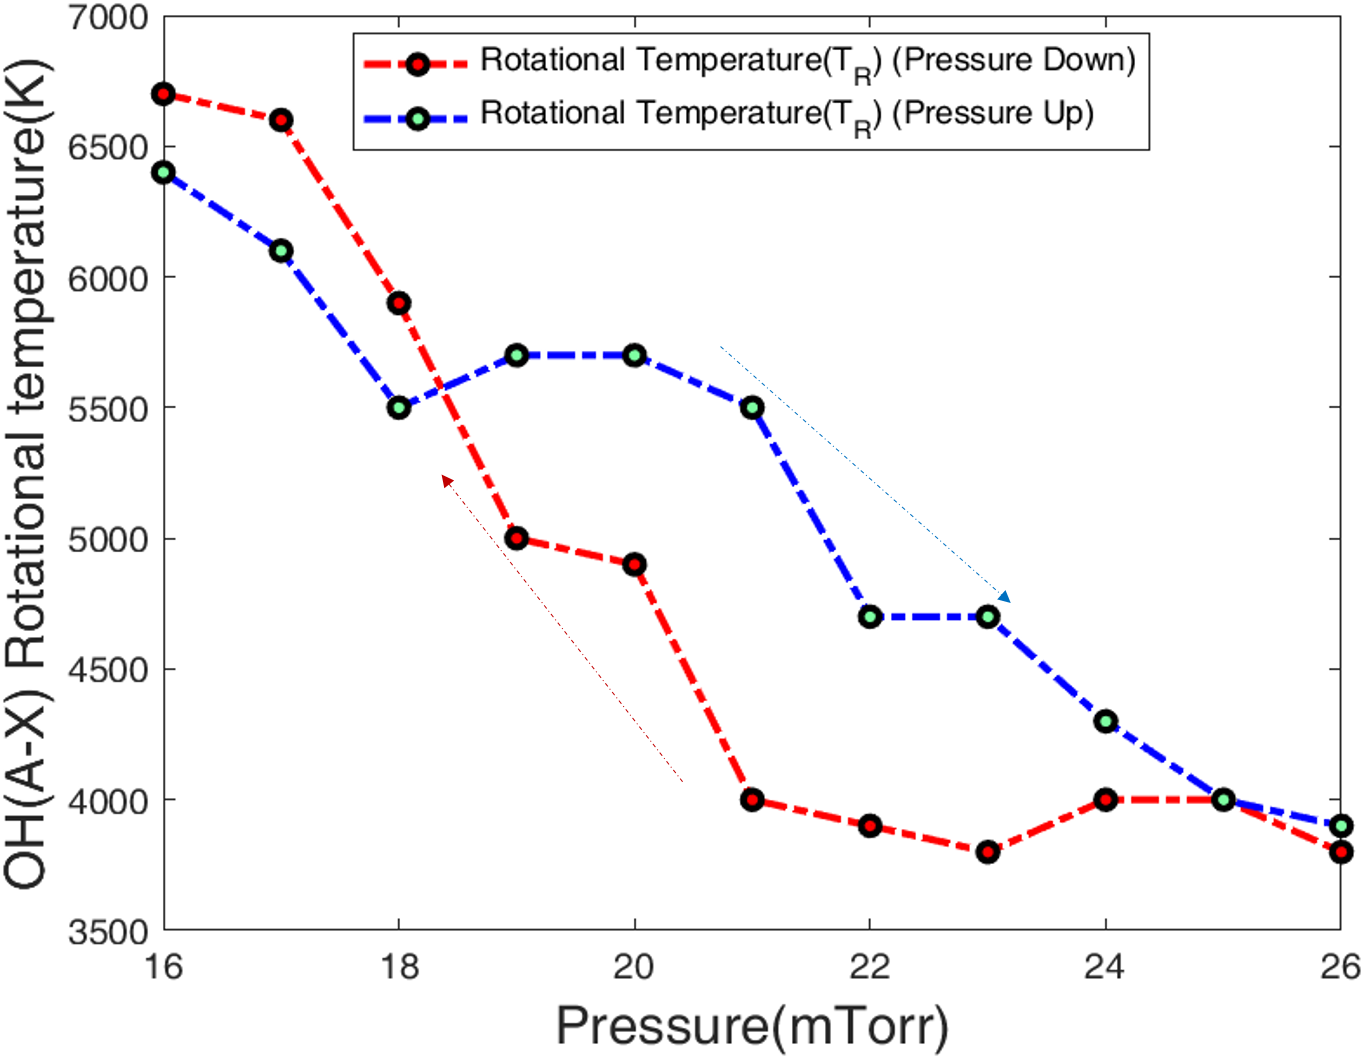}
    \caption{The rotational temperature measured by the OH (A-X) emission lines using the monochromator. This result verifies the hysteresis of rotational temperature obtained by OES.}
    \label{fig:iccd_rot}
\end{figure}

\begin{figure}[h!]
    \centering
    \includegraphics[width = 164.6 mm]{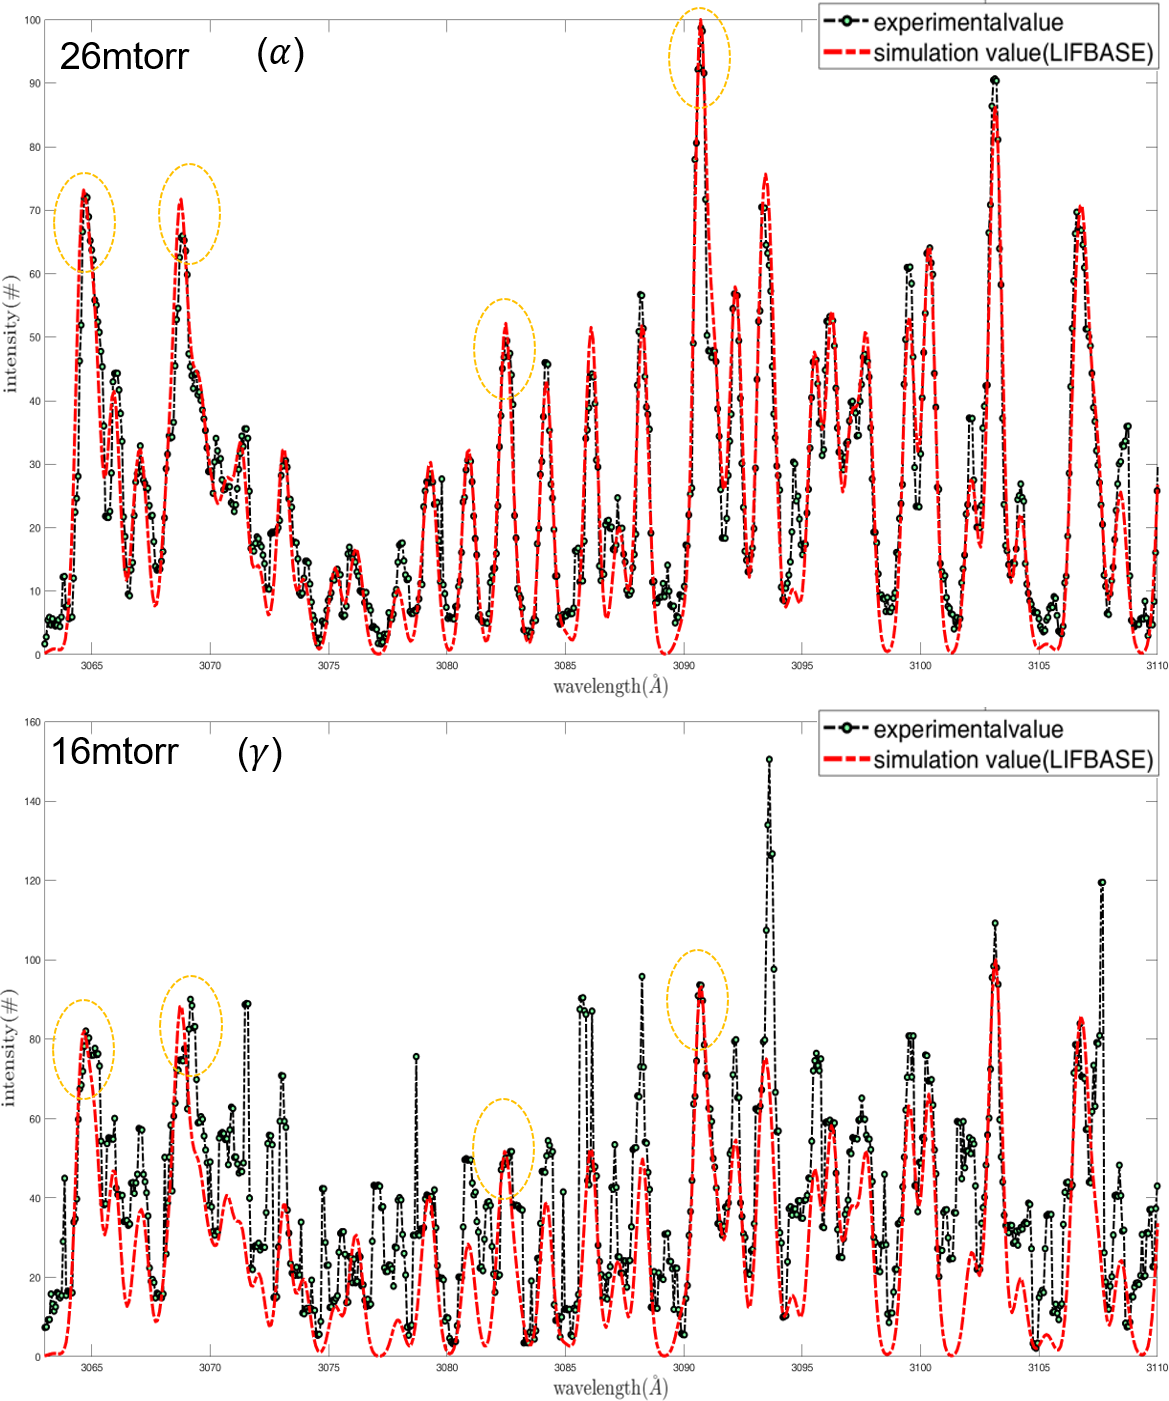}
    \caption{Examples of fittings between experimental values and LIFBASE data (red line: LIFBASE data, black line: experimental data).}
    \label{fig:fitting_iccd}
\end{figure}
\FloatBarrier

\begin{figure}[h!]
    \centering
    \includegraphics[width = 164.6 mm]{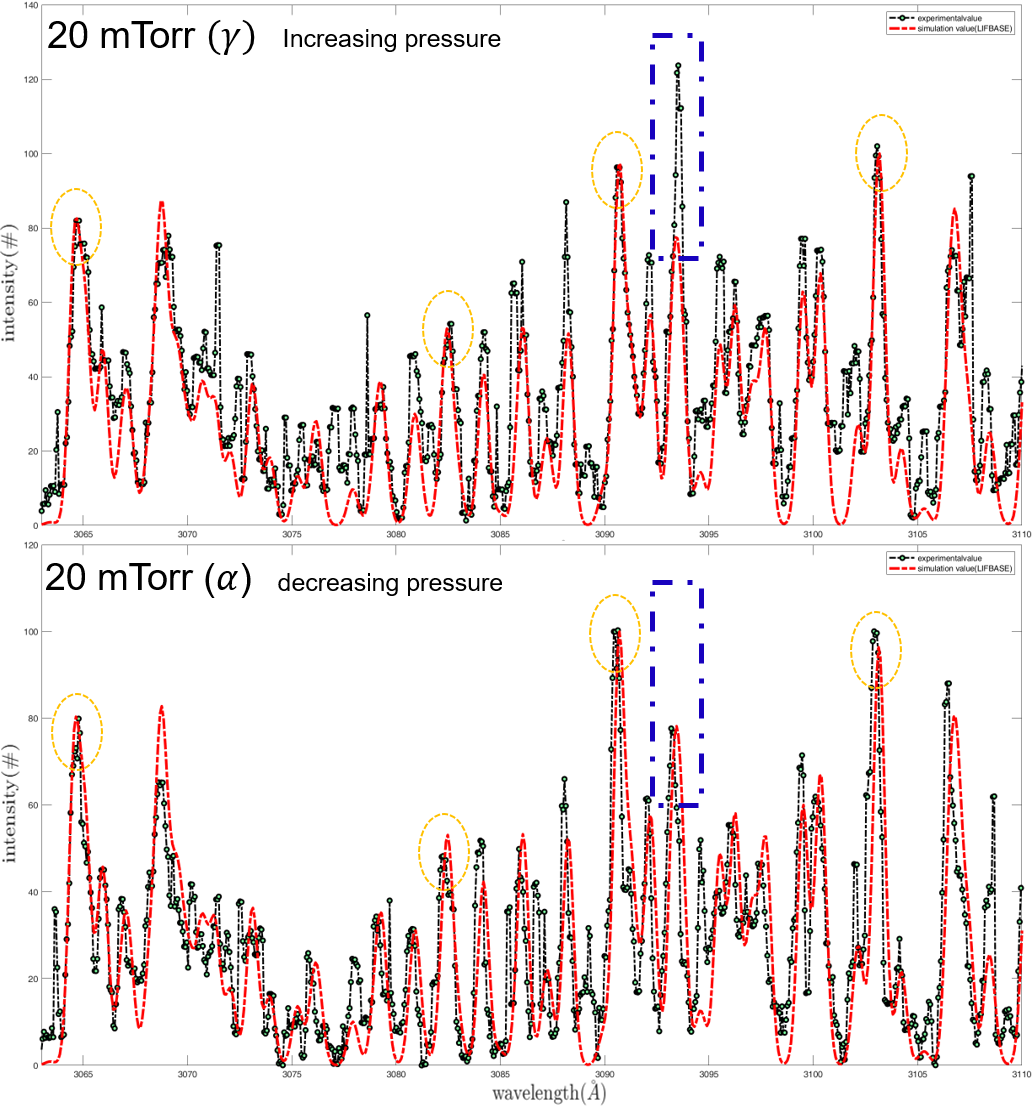}
    \caption{The comparison of data with the same operating parameters (pressure, power, gas composition and electrode) under increasing and decreasing pressure. There are two different stable states: $\gamma$ mode and $\alpha$ mode. We can distinguish the states through the existence of a representative Ar II emission peak (the blue box). (red line: LIFBASE data, black line: experimental data).}
    \label{fig:compare_20mtorr}
\end{figure}
\FloatBarrier
